# Supplementary material for: Universal Scaling of Polygonal Desiccation Crack Patterns
Source: arXiv:1807.06126 ancillary file (2018-11-29)
Supplement: Supplementary file 1 [file Supplemental_Material.pdf]

# Supplemental Material:
# “Universal Scaling of Polygonal Desiccation Crack Patterns”


Xiaolei Ma,* Janna Lowensohn, and Justin C. Burton

*Department of Physics, Emory University, Atlanta, Georgia 30322, USA*



(Dated: November 29, 2018)


## I. SUPPLEMENTAL VIDEOS

We provide three supplemental videos. The details of each video are as follows:

•Video_S1. This video shows the formation of hierarchical crack patterns during drying cornstarch-water suspensions with initial volume fraction $\phi_i = 40\%$ in a petri dish. The duration of the video in real time is 3 days.

•Video_S2. This video shows the formation of polygonal crack patterns during drying cornstarch-water suspensions with initial volume fraction $\phi_i = 26\%$ in a thin chamber with thickness $h \approx 750$ $\mu$m. The duration of the video in real time is 3 days.

•Video_S3. This video shows the formation of dentritic crack patterns during drying cornstarch-water suspensions with initial volume fraction $\phi_i = 26\%$ in a thin chamber with thickness $h \approx 10$ $\mu$m. The duration of the video in real time is 1 day.

## II. EFFECT OF SUBSTRATE BOUNDARY CONDITIONS ON CRACK FORMATION

The stress boundary condition at substrate can potentially play a role in the formation of desiccation crack patterns. We examined the effect of the boundary condition on the formation of crack patterns by drying cornstarch-water suspensions in petri dishes. We modified the bottom surfaces of the petri dishes: silicon carbide sheets were used to roughen the petri dish surface; a commercial coating (Rain-X) was applied in order to make the surface more hydrophobic; and an epoxy resin layer was applied to the petri dish to enhance the adhesive properties.

We prepared cornstarch-water suspensions with the same initial volume ($V_i = 120$ ml) and the same initial volume fractions ($\phi_i = 40\%$), then deposited the suspensions into the prepared petri dishes with different boundary conditions, and the suspensions dried at room temperature. Figure


* xiaolei.ma@emory.edu

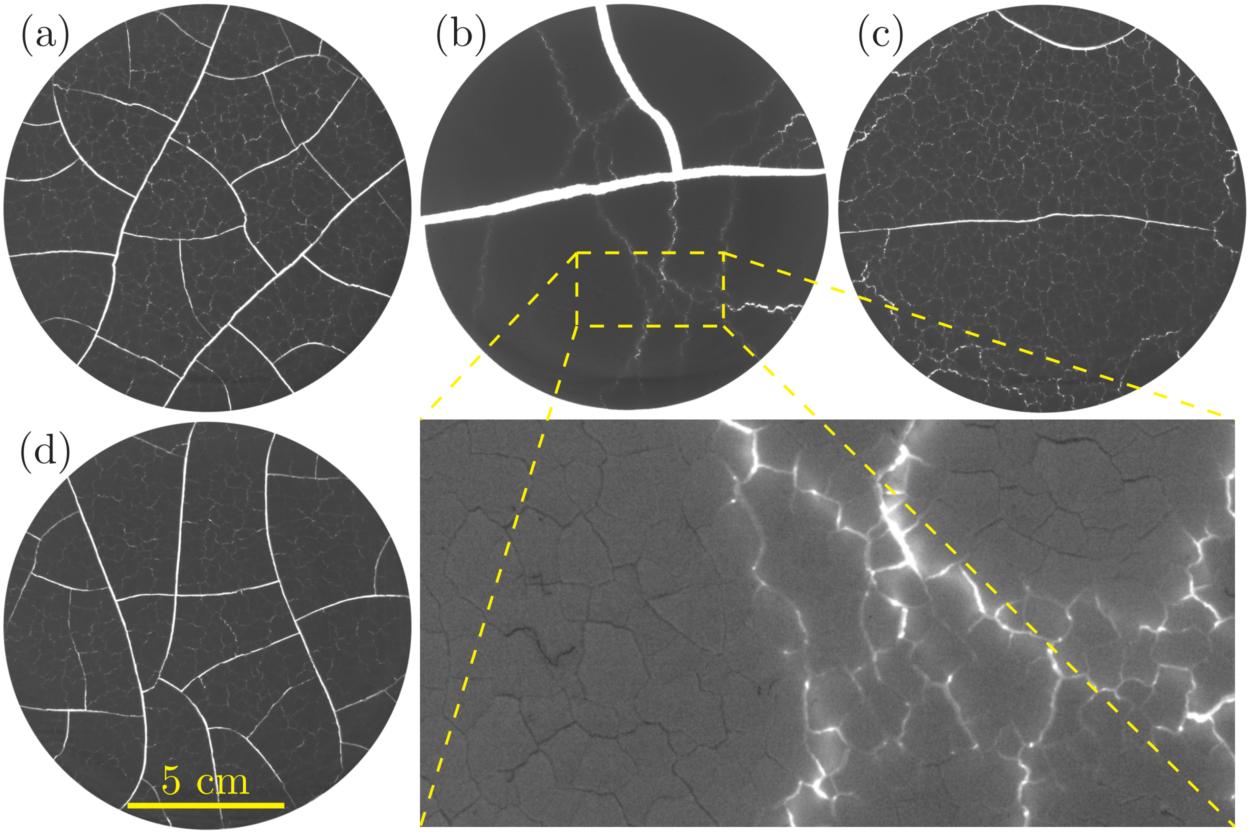


FIG. S1. Desiccation crack patterns of cornstarch-water suspensions with the same initial volume ($V_i$ = 120 ml) and the same initial volume fraction ($\phi_i$ = 40%) dried in petri dishes with different boundary conditions. (a) Image of the dried polygonal cracks without modifying the surfaces of the petri dish. (b) The surface of the petri dish was roughened by silicon carbide sheets. (c) The surface of the petri dish was made hydrophobic by coating with a layer of Rain-X. (d) The surface of the petri dish was coated with an epoxy resin layer. The scale bar applies to all images. The zoomed-in image of (b) was enhanced for better visualization of secondary, small-scale cracks.

S1a shows the crack patterns of the dried cornstarch-water film without any modification to the petri dish surface as a control experiment. It is evident that the increase of the surface roughness will decrease the number of large-scale cracks as indicated by Fig. S1b, and the small-scale cracks are still observable as shown in the zoomed-in image of a particular region enclosed by a dashed yellow box in Fig. S1b. Similarly, as the hydrophobicity was increased (Fig. S1c), the number of large-scale cracks dramatically decreased, whereas the small-scale cracks are insensitive to the coating layer. The results shown in Fig. S1b and S1c indicate that the decrease in adhesion of the suspension to the substrate leads to dramatic decrease in the number of large-scale, primary cracks (or the increase of polygon area), which is likely due to the more isotropic shrinkage of the film

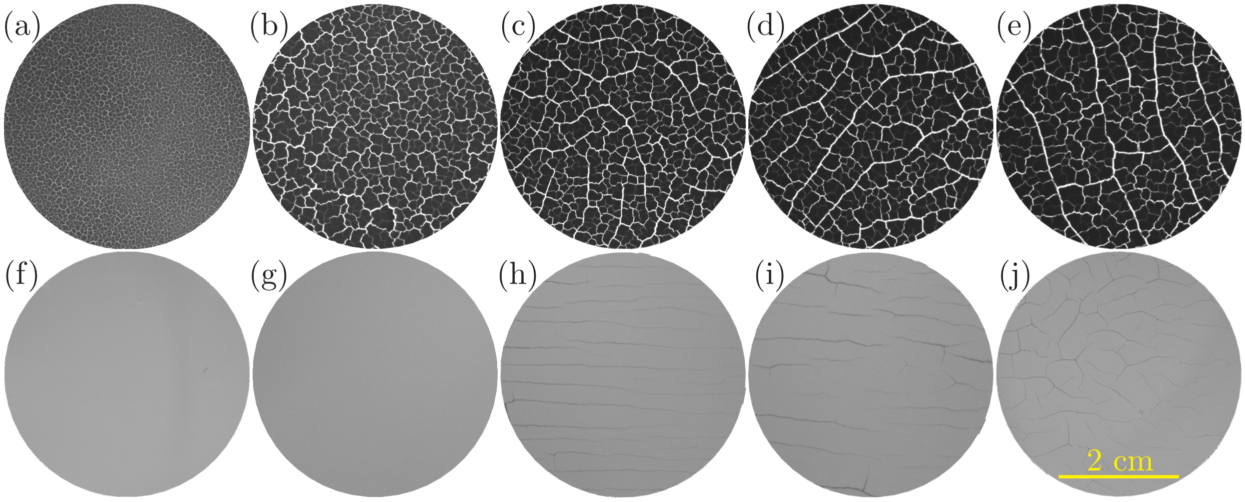


FIG. S2. Measurement of critical film thickness for cracking of cornstarch-water and $CaCO_3$-water suspensions. Images (a) to (e) show dried cornstarch-water suspensions with thicknesses of 281 $\mu$m, 600 $\mu$m, 864 $\mu$m, 1181 $\mu$m, and 1236 $\mu$m, respectively. Images (f) to (j) show dried $CaCO_3$-water suspensions with thicknesses of 267 $\mu$m, 500 $\mu$m, 553 $\mu$m, 635 $\mu$m, and 701 $\mu$m, respectively. The scale bar applies to all images.

during drying.

Figure S1d shows the polygonal cracks in a petri dish whose surface was coated with an epoxy resin layer. In this case, although the adhesion of the suspension to the substrate has increased, the number of large-scale cracks does not dramatically change compared to Fig. S1a. This is not surprising since shrinkage in the film will continue until the yield stress of the granular material is reached so that a crack is formed, and then this process continues. Therefore, although the boundary condition plays a key role in determining the area of the polygonal cracks, weakening the adhesion has the strongest effect, especially if the adhesive stress is smaller than the yield stress of the material.

## III. CRITICAL FILM THICKNESS FOR CRACK FORMATION

We used cornstarch-water and $CaCO_3$-water suspensions to examine whether Eq. (1) in the main text can predict the critical film thickness ($h_c$) for crack formation. The results are shown in Fig. S2. In Fig. S2a-b, only small-scale, secondary cracks are observed. In Fig. S2c, the small-scale, secondary cracks are obvious, and the large-scale, primary cracks are not very apparent, however, are about to appear. In Fig. S2d, both large-scale, primary cracks and small-scale, secondary

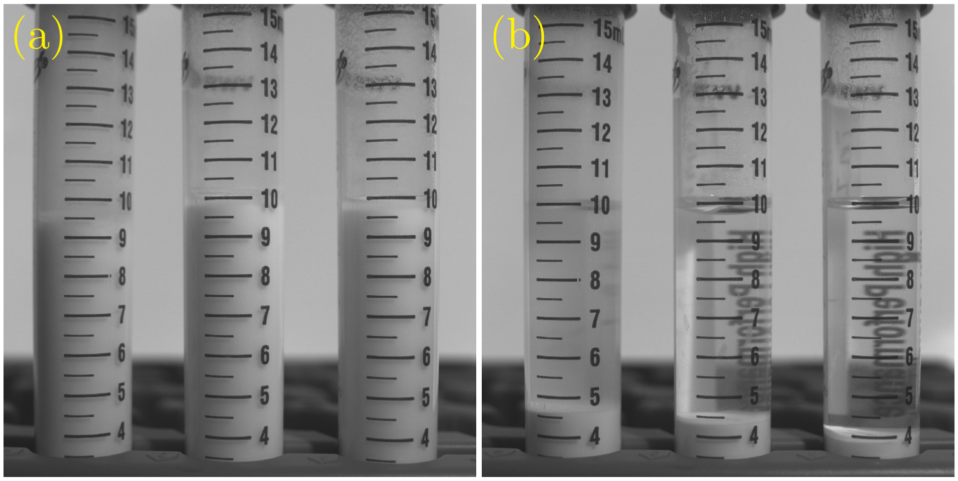


FIG. S3. Suspensions of cornstarch-silicone oil, cornstarch-water, and cornstarch-IPA (from left to right) with the same same initial volume ($V_i$ = 10 ml), and the same initial volume fraction ($\phi_i$ = 20%). (a) and (b) show the images of the initial suspensions and the suspensions after being centrifuged, respectively.

cracks are obvious. This indicates that the critical film thickness for large-scale, primary cracks of cornstarch-water suspensions lies in between $h = 864$ $\mu$m (Fig. S2c) and $h = 1181$ $\mu$m (Fig. S2d), which agrees fairly well with the prediction by Eq. (1) ($h_c \approx 1500$ $\mu$m). In Fig. S2g, no cracks are visible, whereas in Fig. S2h cracks appear, suggesting that the critical film thickness for primary cracks of $CaCO_3$-water suspensions lies in between 500 $\mu$m and 553 $\mu$m, which again agrees with the prediction by Eq. (1) ($h_c \approx 400$ $\mu$m).

## IV. PACKING ABILITY OF DIFFERENT PARTICLE-LIQUID COMBINATIONS

In order to examine the role of the suspending liquids in the desiccation crack patterns, we measured the packing abilities of cornstarch particles suspended in different liquids. We prepared cornstarch-water, cornstarch-silicone oil, and cornstarch-IPA suspensions with the same initial volume ($V_i$ = 10 ml), and the same initial volume fraction ($\phi_i$ = 20%). The samples were then centrifuged at 2000 rpm for 2 mins. Longer centrifuge times did not change the result.

According to particle number conservation,

$$\phi_f V_f = \phi_i V_i, \tag{S1}$$

where $\phi_f$ and $V_f$ are the final volume fraction and the total volume of the particle suspension after being centrifuged, respectively. Figure S3a shows images of the initial cornstarch suspensions, and the images of the cornstarch suspensions after being centrifuged are shown in Fig. S3b. From Fig.

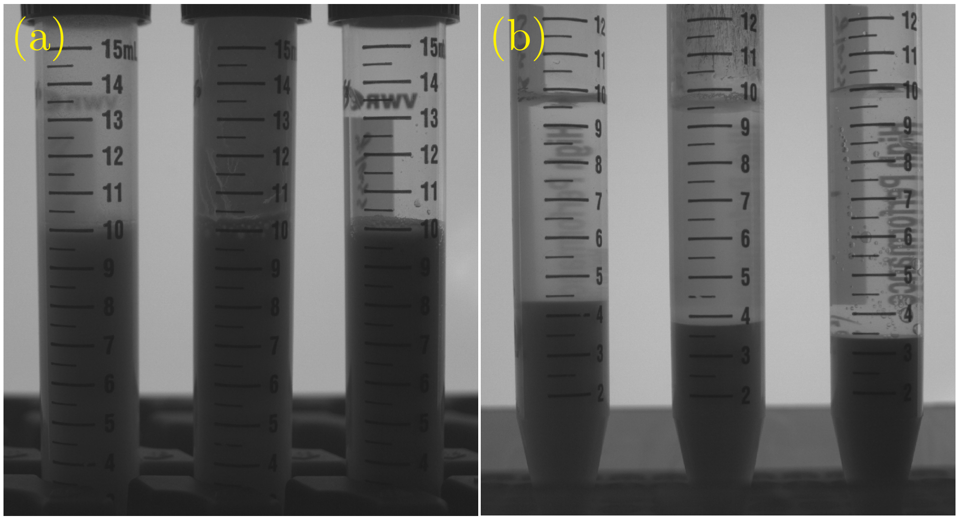


FIG. S4. Suspensions of cornstarch-water, $CaCO_3$-water, and glass beads-water (from left to right) with the same initial volume fraction ($\phi_i = 20\%$), and the same initial volume ($V_i$= 10 ml). (a) and (b) show the images of the initial suspensions and images of the suspensions after being centrifuged, respectively.

S3b we find that $V_f \approx 4.6$ ml, 4.4 ml, and 3.9 ml for cornstarch particles in silicone oil, water, and IPA, respectively. Therefore, we can calculate that $\phi_f \approx 43\%$ for cornstarch-silicone oil, $\phi_f \approx 45\%$ for cornstarch-water, and $\phi_f \approx 51\%$ for cornstarch-IPA, respectively.

Additionally, we measured the packing abilities of different particles suspended in water. To do this, we prepared the suspensions of cornstarch-water, $CaCO_3$-water, and glass beads-water with the same initial volume ($V_i = 10$ ml), and the same initial volume fraction ($\phi_i = 20\%$) as shown in Fig. S4a from left to right, respectively. Figure S4b shows the images of the three suspensions after being centrifuged. From Fig. S4b, we can obtain the the final volume $V_f$ of different particles in water, i.e., $V_f \approx 4.4$ ml for cornstarch, $V_f \approx 3.8$ ml for $CaCO_3$, and $V_f \approx 3.4$ ml for glass beads. Therefore, using Eq. S1 we can calculate the final volume fraction $\phi_f$ for different particles in water, i.e., $\phi_f \approx 45\%$ for cornstarch, $\phi_f \approx 53\%$ for $CaCO_3$, and $\phi_f \approx 59\%$ for glass beads. We can conclude that the packing efficiency of a specific material can be significantly different in different liquids, and can potentially affect the modulus of the material and the visibility of the cracks, among other properties.

## V. EFFECT OF INITIAL VOLUME FRACTION ON CRACK SIZE

We prepared cornstarch-water suspensions with different initial volume fractions $\phi_i$, and dried the suspensions in thin chambers. Figure S5 shows the variations of crack area $A_p$ with respect

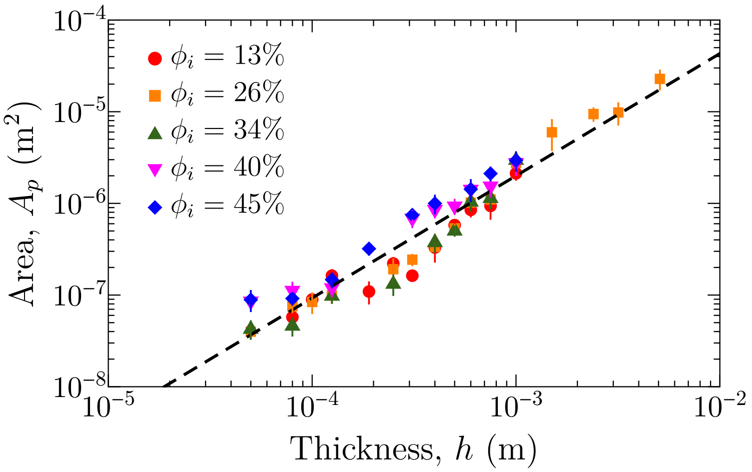


FIG. S5. Scaling behavior of polygon area $A_p$ vs. film thickness $h$ for cornstarch-water suspensions with various initial volume fractions $\phi_i$. The dashed black line represents the best fit for the data, $A_p = 0.02$ m$^{2/3}$ $h^{4/3}$. The error bars are from the standard deviation of multiple measurements. The same data is shown in Fig. 8 of the main text (black points).

to the film thickness $h$ (chamber thickness) for cornstarch-water suspensions with various initial volume fractions. It is evident that the data of $A_p$ and $h$ for different $\phi_i$ collapse onto a single curve $A_p = 0.02$ m$^{2/3}$ $h^{4/3}$ as indicated by the dashed black line, suggesting that the initial volume fraction $\phi_i$ does not influence the crack size.

## VI. MODULUS MEASUREMENTS

We used the indentation load-displacement method to measure the Young's modulus of particulate films as described in the main text. In addition to the measurement of the films shown in Fig. 10, we also measured Young's modulus of the fully desiccated particulate films, and the results are shown in Fig. S6. Using Eq. 7 in the main text to fit the unloading data in Fig. S6, the modulus of fully-desiccated films is calculated to be as follows: $1.6 \times 10^7$ Pa (cornstarch-IPA film, see Fig. S6a), $2.1 \times 10^6$ Pa (cornstarch-water film, see Fig. S6b), $2.0 \times 10^7$ Pa (cornstarch-silicone oil film, see Fig. S6c), $2.1 \times 10^8$ Pa ($CaCO_3$-water, see Fig. S6d). The errors of the nonlinear fit using Eq. 7 range from 0.4% to 2%. From Figs. 10 and S6, one can tell the Young's modulus of fully-desiccated $CaCO_3$-water and cornstarch-water films is of the same order of magnitude to their wet counterparts.

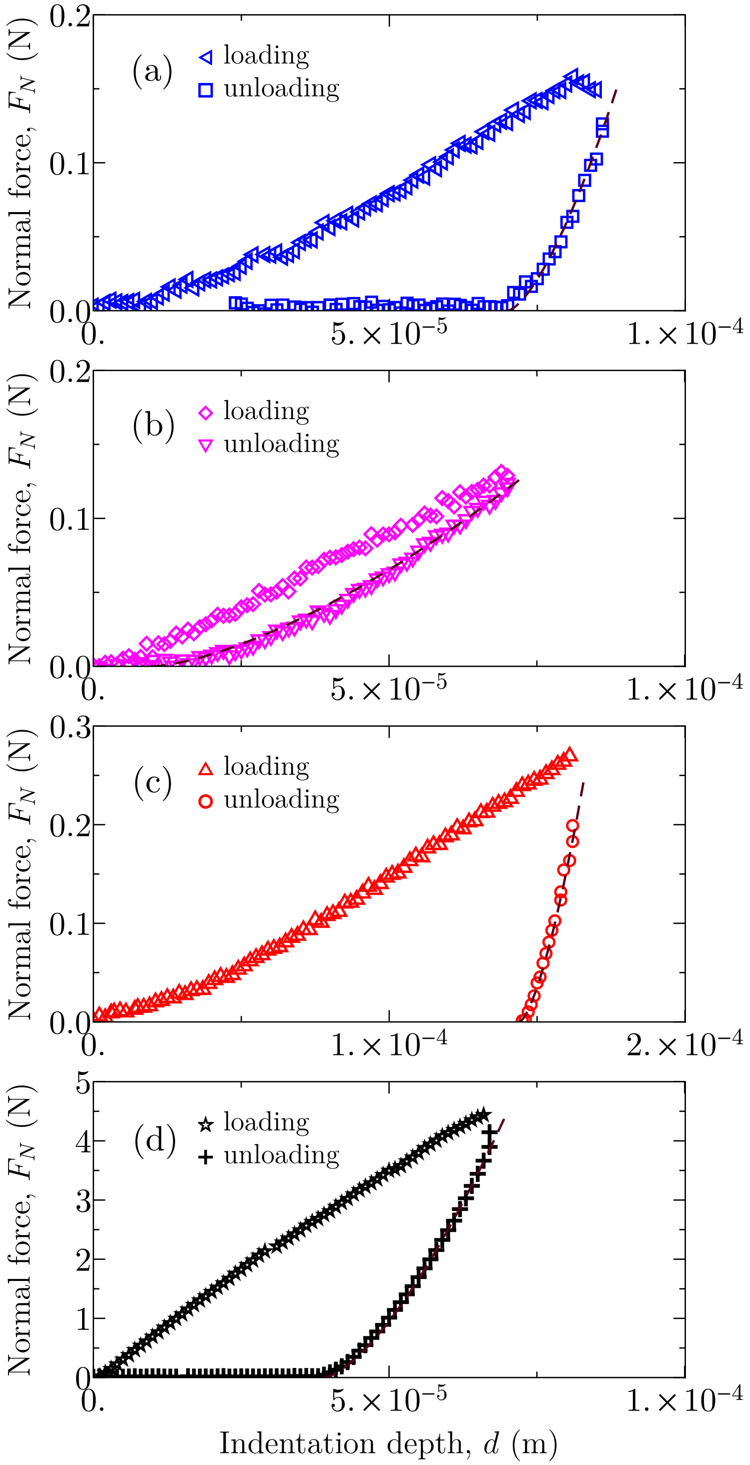


FIG. S6. Indentation-loading displacement tests of different films at different drying stages. (a), (b), (c) and (d) show the data on fully-desiccated cornstarch-IPA film, cornstarch-water film, cornstarch-silicone oil film, and $CaCO_3$-water film, respectively. The dashed lines represent the best fits of the unloading data using Eq. 7 in the main manuscript.

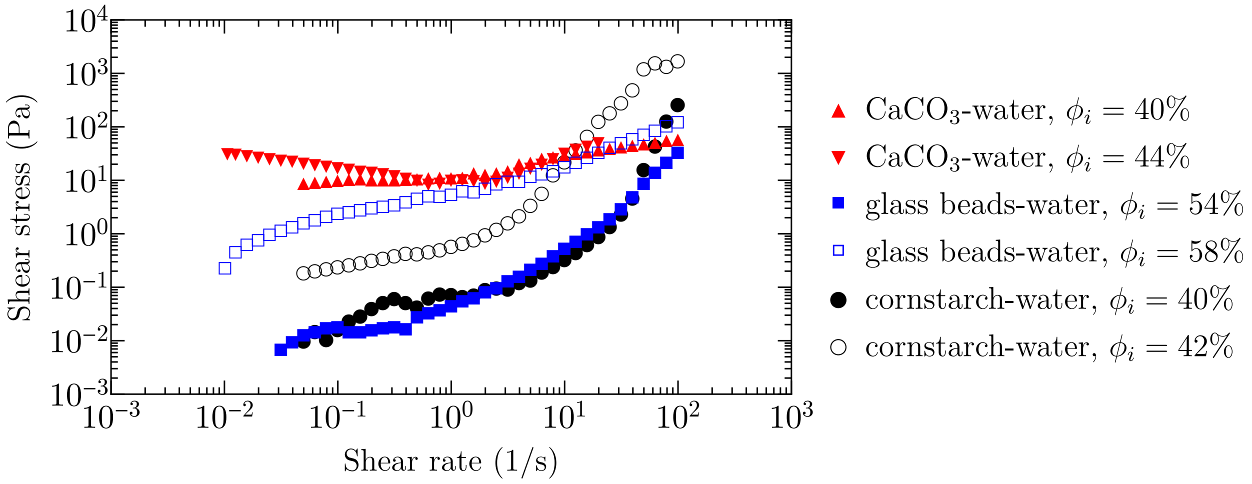


FIG. S7. Rheology measurements of particulate suspensions with different initial volume fractions $\phi_i$.

## VII. RHEOLOGICAL MEASUREMENTS

In order to examine the role of particle-particle interactions, we also measured the rheological properties of cornstarch-water, $CaCO_3$-water and glass beads-water suspensions with different initial volume fractions $\phi_i$, and the results are shown in Fig. S7. Measurements were performed using a flat, stainless steel tool in a TA Instruments AR2000 rheometer. Although shear thickening is observed in more concentrated suspensions, the maximum shear stress ($\sim 10^3$ Pa) is smaller than the capillary stress ($\gamma/R \sim 15$ kPa for cornstarch-water). This strongly suggests that capillary forces are larger than any inter-particle forces in the bulk suspension.
